# Supplementary material for: SCOT: Self-Supervised Contrastive Pretraining For Zero-Shot Compositional Retrieval
Source: arXiv:2501.08347 source file (2025-01-12)
Supplement: Supplementary file 1 [file fashionIQ_main_results.tex]

\begin{table*}[t]
\centering
\setlength{\tabcolsep}{2.8pt}
\fontsize{6.5pt}{4.5pt}\selectfont
\begin{tabular}{p{0.5cm}llp{0.65cm}p{0.65cm}p{0.65cm}p{0.65cm}p{0.65cm}p{0.65cm}p{0.65cm}p{0.65cm}}
\toprule
\multirow{2}{*}{\textbf{}} & \multirow{2}{*}{\textbf{Method}} & \multirow{2}{*}{\textbf{Venue}} & \multicolumn{2}{c}{\textbf{Average}} & \multicolumn{2}{c}{\textbf{Dress}} & \multicolumn{2}{c}{\textbf{Shirt}} & \multicolumn{2}{c}{\textbf{Top/Tee}}\\
\cmidrule(lr){4-5} \cmidrule(lr){6-7} \cmidrule(lr){8-9} \cmidrule(lr){10-11}
& & & $\boldsymbol{R @ 10}$ & $\boldsymbol{R @ 50}$ & $\boldsymbol{R @ 10}$ & $\boldsymbol{R @ 50}$ & $\boldsymbol{R @ 10}$ & $\boldsymbol{R @ 50}$ & $\boldsymbol{R @ 10}$ & $\boldsymbol{R @ 50}$\\
\midrule
\multirow{4}{*}{Sup.}
& DCNet \cite{dcnet} & AAAI'21 & 30.44 & 58.29 & 28.95 & 56.07 & 23.95 & 47.30 & 30.44 & 58.29\\ 
& CLIP4CIR \cite{combinerarch} & CVPR'22 & 38.32 & 61.74 & 33.81 & 59.40 & 39.99 & 60.45 & 41.41 & 65.37\\
& FashionVLP \cite{fashionVLP} & CVPR'23 & 34.27 & 62.51 & 32.42 & 60.29 & 31.89 & 58.44 & 38.51 & 68.79\\
& BLIP4CIR \cite{BLIP4Cir} & Preprint & 43.49 & 67.31 & 42.09 & 67.33 & 41.76 & 64.28 & 46.61 & 70.32\\
\midrule
\multirow{8}{*}{Z-S}
& PALAVRA \cite{PALAVRA} & ICCV'22 & 19.76 & 37.25 & 17.25 & 35.94 & 21.49 & 37.05 & 20.55 & 38.76 \\
& Pic2Word \cite{Saito_2023_CVPR} & CVPR'23 & 24.7 & 43.7 & 20.0 & 40.2 & 26.2 & 43.6 & 27.9 & 47.4 \\
& SEARLE-XL-OTI \cite{SEARLE} & ICCV'23 & 27.61 & 47.9 & 21.57 & 44.47 & 30.37 & 47.49 & 30.9 & 51.76\\

& Context-I2W \cite{tang2023context} & Preprint & 27.8 & 48.9 & 23.1 & 45.3 & 29.7 & 48.6 & 30.6 & 52.9\\
& Chen et al., 2023 \cite{chen2023pretrain} & Preprint & 38.63 & 58.51 & 28.11 & 51.12 & 39.42 & \textbf{62.68} & 35.39 & 57.44\\

& CompoDiff (ViT-L) \cite{gu2023compodiff} & Preprint & 37.36 & 50.85 & 33.91 & 47.85 & 38.1 & 52.48 & 40.07 & 52.22 \\
& CompoDiff (ViT-G) \cite{gu2023compodiff} & Preprint & \textbf{39.02} &  51.71 & \textbf{37.78} & 49.10 & 41.31 &  55.17 & \textbf{44.26} & 56.41 \\

& SCOT (Ours) & Ours & 38.45 & \textbf{60.03} & 32.78 & \textbf{55.91} & \textbf{41.42} & 61.09 & 41.15 & \textbf{63.10} \\
\bottomrule
\end{tabular}
\vspace{0.5em}
\caption{\textbf{Results on FashionIQ.} 
The bottom portion of the table presents zero-shot results from our proposed approach compared against existing zero-shot methods, while the top portion presents results from existing fully-supervised approaches.
}
\label{table:fashioniq_full}
\vspace{-1em}
\end{table*}
