# Supplementary material for: SCOT: Self-Supervised Contrastive Pretraining For Zero-Shot Compositional Retrieval
Source: arXiv:2501.08347 source file (2025-01-12)
Supplement: Supplementary file 2 [file cirr_backbone_analysis.tex]

% Please add the following required packages to your document preamble:
% \usepackage{multirow}
\begin{table*}[]
\centering
\begin{tabular}{llccccccc}
\toprule
\multirow{2}{*}{} & \multirow{2}{*}{\textbf{Method}} & \multicolumn{4}{c}{\textbf{Recall@K}} & \multicolumn{3}{c}{\textbf{Recall$_{\text{subset}}$@K}} \\
\cmidrule(lr){3-6} \cmidrule(lr){7-9}
 & & \( K = 1 \) & \( K = 5 \) & \( K = 10 \) & \( K = 50 \) & \( K = 1 \) & \( K = 2 \) & \( K = 3 \) \\
\midrule
\multirow{4}{*}{CLIP ViT-B/32}
& Image-Only & 6.94 & 22.94 & 33.71 & 59.18 & 21.06 & 41.01 & 60.34 \\
& Text-Only & 21.16 & 45.35 & 57.40 & 81.06 & \textbf{62.26} & \textbf{81.08} & \textbf{90.75} \\
& Image+Text & 10.46 & 32.41 & 46.39 & 75.11 & 30.09 & 54.24 & 73.20 \\
& SCOT & \textbf{22.80} & \textbf{53.18} & \textbf{66.22} & \textbf{89.64} & 53.25 & 75.45 & 88.31 \\
\midrule
\multirow{4}{*}{CLIP ViT-L/14}
& Image-Only & 7.47 & 23.88 & 34.07 & 57.57 & 20.87 & 41.95 & 61.13 \\
& Text-Only & 22.00 & 45.79 & 57.57 & 79.59 & \textbf{61.71} & \textbf{80.26} & \textbf{90.43} \\
& Image+Text & 10.55 & 32.70 & 45.71 & 74.26 & 31.06 & 55.69 & 73.93 \\
& SCOT & \textbf{24.36} & \textbf{53.52} & \textbf{67.37} & \textbf{89.35} & 51.47 & 74.24 & 87.90 \\
\midrule
\multirow{4}{*}{BLIP-2}
& Image-only & 7.59 & 24.43 & 35.56 & 61.42 & 20.74 & 40.67 & 61.08 \\
& Text-only & 33.52	& 61.50 & 71.35 & 88.31 & 72.53 & 88.02 & \textbf{94.87} \\
& Image + Text & 19.69 & 49.98 & 64.39 & 90.01 & 45.69 & 71.18 & 85.83 \\
& SCOT (Ours) & \textbf{36.82} & \textbf{64.34} & \textbf{74.48} & \textbf{93.42} & \textbf{75.73} & \textbf{88.70} & 94.84 \\
\bottomrule
\end{tabular}
\caption{\textbf{Results on CIRR.} Zero-shot results on CIRR while varying the image-text encoders.}
\label{table:cirr_backbone}
%\vspace{-1.0em}
\end{table*}
