# Supplementary material for: SCOT: Self-Supervised Contrastive Pretraining For Zero-Shot Compositional Retrieval
Source: arXiv:2501.08347 source file (2025-01-12)
Supplement: Supplementary file 3 [file cirr_main_results.tex]

\begin{table*}[]
\setlength{\tabcolsep}{2.8pt}
\fontsize{6.5pt}{4.5pt}\selectfont
\centering
\begin{tabular}{lllccccccc}
\toprule
\multirow{2}{*}{} & \multirow{2}{*}{\textbf{Method}} & \multirow{2}{*}{\textbf{Venue}} & \multicolumn{4}{c}{\textbf{Recall@K}} & \multicolumn{3}{c}{\textbf{Recall$_{\text{subset}}$@K}} \\
\cmidrule(lr){4-7} \cmidrule(lr){8-10}
 & & & \( K = 1 \) & \( K = 5 \) & \( K = 10 \) & \( K = 50 \) & \( K = 1 \) & \( K = 2 \) & \( K = 3 \) \\
\midrule
\multirow{4}{*}{Sup.}
& MAAF \cite{maaf} & Preprint & 10.31 & 33.03 & 48.30 & 80.06 & 21.05 & 41.81 & 61.60 \\
& CIRPLANT \cite{CIRR} & ICCV'21 & 19.55 & 52.55 & 68.39 & 92.38 & 39.20 & 63.03 & 79.49 \\
& CLIP4CIR \cite{combinerarch} & CVPR'22 & 33.59 & 65.35 & 77.35 & 95.21 & 62.39 & 81.81 & 92.02 \\
& BLIP4CIR \cite{BLIP4Cir} & Preprint & 40.15 & 73.08 & 83.88 & 96.27 & 72.10 & 88.27 & 95.93 \\
\midrule
\multirow{9}{*}{Z-S} 
% & Image-only & - & 7.59 & 24.43 & 35.56 & 61.42 & 20.74 & 40.67 & 61.08 \\
% & Text-only & - & 33.52	& 61.50 & 71.35 & 88.31 & 72.53 & 88.02 & 94.87 \\
% & Image + Text & - & 19.69 & 49.98 & 64.39 & 90.01 & 45.69 & 71.18 & 85.83 \\

& PALAVRA \cite{PALAVRA} & ECCV'22 & 16.62 & 43.49 & 58.51 & 83.95 & 41.61 & 65.30 & 80.94 \\
& Pic2Word \cite{Saito_2023_CVPR} & CVPR'23 & 23.9 & 51.7 & 65.3 & 87.8 & - & - & - \\
& SEARLE-XL-OTI \cite{SEARLE} & ICCV'23 & 24.87 & 52.31 & 66.29 & 88.58 & 53.80 & 74.31 & 86.94 \\

& CIReVL \cite{trainingfree} & Preprint & 24.55 & 52.31 & 64.92 & 86.34 & 59.54 & 79.88 & 89.69 \\
& Context-I2W~\cite{tang2023context} & Preprint & 25.6 & 55.1 & 68.5 & 89.8 & - & - & -\\ 
& Chen et al., 2023 \cite{chen2023pretrain} & Preprint & 25.52 & 54.58 & 67.59 & 88.70 & 55.64 & 77.54 & 89.47\\ 

& CompoDiff (ViT-L) \cite{gu2023compodiff} & Preprint & 22.35 & 54.36 & 73.41 & 91.77 & 35.84 & 56.11 & 76.60\\
& CompoDiff (ViT-G) \cite{gu2023compodiff} & Preprint & 26.71 & 55.14 & \textbf{74.52} & 92.01 & 64.54 & 82.39 & 91.81\\

& SCOT (Ours) & Ours & \textbf{36.82} & \textbf{64.34} & 74.48 & \textbf{93.42} & \textbf{75.73} & \textbf{88.70} & \textbf{94.84} \\
\bottomrule
\end{tabular}
\vspace{0.5em}
\caption{\textbf{Results on CIRR.} 
%$\text{*}$ are the results reported by the authors.
The bottom portion of the table presents zero-shot results from our proposed approach compared against existing zero-shot methods, while the top portion presents results from existing fully-supervised approaches.}
\label{table:cirr_full}
\vspace{-1.0em}
\end{table*}
