# Supplementary material for: SCOT: Self-Supervised Contrastive Pretraining For Zero-Shot Compositional Retrieval
Source: arXiv:2501.08347 source file (2025-01-12)
Supplement: Supplementary file 4 [file fiq_backbone_table.tex]

\begin{table*}[]
\centering
\begin{tabular}{llcccccccc}
\toprule
\multirow{2}{*}{\textbf{}} & \multirow{2}{*}{\textbf{Method}} & \multicolumn{2}{c}{\textbf{Average}} & \multicolumn{2}{c}{\textbf{Dress}} & \multicolumn{2}{c}{\textbf{Shirt}} & \multicolumn{2}{c}{\textbf{Top/Tee}} \\
\cmidrule(lr){3-4} \cmidrule(lr){5-6} \cmidrule(lr){7-8} \cmidrule(lr){9-10}
& & $\boldsymbol{R @ 10}$ & $\boldsymbol{R @ 50}$ & $\boldsymbol{R @ 10}$ & $\boldsymbol{R @ 50}$ & $\boldsymbol{R @ 10}$ & $\boldsymbol{R @ 50}$ & $\boldsymbol{R @ 10}$ & $\boldsymbol{R @ 50}$ \\
\midrule
\multirow{4}{*}{CLIP ViT-B/32}
& Image-Only & 5.88 & 13.19 &  6.96 & 14.08 & 4.46 & 11.89 & 6.22 & 13.61 \\ 
& Text-Only & 18.41 & 36.28 & 14.92 & 33.81 & 19.77 & 34.69 & 20.55 & 40.33 \\
& Image+Text & 13.36 & 27.51 &  12.44 & 28.55 & 12.61 & 24.82 & 15.04 & 29.16  \\
& SCOT & \textbf{24.14} & \textbf{43.44} & \textbf{19.73} & \textbf{41.24} & \textbf{25.51} & \textbf{42.93} & \textbf{27.18} & \textbf{46.14}  \\
\midrule
\multirow{4}{*}{CLIP ViT-L/14}
& Image-Only & 7.97 & 17.43 & 5.25 & 13.63 & 10.54 & 20.65 & 8.10 & 18.01  \\ 
& Text-Only & 19.01 & 35.26 & 15.22 & 33.01 & 19.82 & 33.31 & 21.87 & 39.46 \\
& Image + Text & 18.12 & 33.17 & 14.27 & 31.33 & 19.13 & 32.28 & 20.95 & 35.90 \\
& SCOT & \textbf{28.27} & \textbf{47.44} & \textbf{23.69} & \textbf{45.06} & \textbf{29.09} & \textbf{47.01} & \textbf{32.02} & \textbf{50.33}  \\
\midrule
% \multirow{4}{*}{CLIP R50x4}
% & Image-Only & - & - &  - & - &  - &  - &  - & - & \\ 
% & Text-Only & - & - &  - & - &  - &  - &  - & - & \\
% & Image+Text & - & - &  - & - &  - &  - &  - & - & \\
% & SCOT & - & - &  - & - &  - &  - &  - & - &  \\
% \midrule
\multirow{4}{*}{BLIP-2}
& Image-Only & 7.53 & 17.93 & 4.21 & 11.89 & 10.59 & 23.51 & 7.81 & 18.41 \\
& Text Only & 24.68 & 43.59 & 20.77 & 41.64 & 25.95 & 42.83 & 27.33 & 46.31  \\
& Image + Text & 29.21 & 50.05 & 23.30 & 45.61 & 32.82 & 53.09 & 31.51 & 51.45  \\
& SCOT (Ours) & \textbf{38.45} & \textbf{60.03} & \textbf{32.78} & \textbf{55.91} & \textbf{41.42} & \textbf{61.09} & \textbf{41.15} & \textbf{63.10}  \\
\bottomrule
\end{tabular}
\caption{\textbf{Results on FashionIQ.} Zero-shot results on FashionIQ while varying the image-text encoders.}\label{table:fiq_different_backbones}
\end{table*}
